# Supplementary material for: Sensor-Movement-Robust Angle Estimation for 3-DoF Lower Limb Joints Without Calibration
Source: arXiv:1910.07240 source file (2019-10-16)
Supplement: Supplementary file 1 [file supplementary_information.pdf]

# Supplementary Information

# Sensor-Movement-Robust Angle Estimation for 3-DOF Lower Limb Joints without Calibration

Chunzhi Yi[1], Feng Jiang[2,3], Zhiyuan Chen[4], Baichun Wei[2,3], Hao Guo[1], Xunfeng Yin[5], Fangzhuo Li[5], Chifu Yang[1],

[1] School of Mechatronics Engineering, Harbin Institute of Technology, Harbin, Heilongjiang, 150001, Heilongjiang, China

[2] School of Computer, Harbin Institute of Technology, Harbin, Heilongjiang, 150001, China

[3] Pengcheng Laboratory, Shenzhen, Guangdong, China

[4] School of Computer Science, University of Nottingham, Malaysia

[5] School of Mechanical Engineering, Harbin Engineering University, Heilongjiang, China.

## 1. Supplementary figures and tables

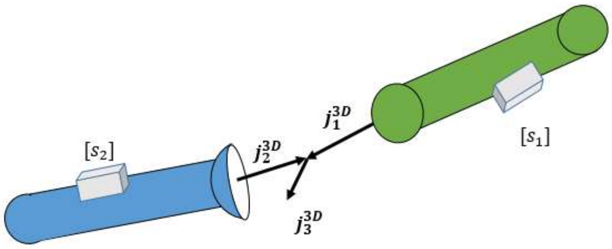

Fig. S1 Three joint axes of a 3-DOF joint.

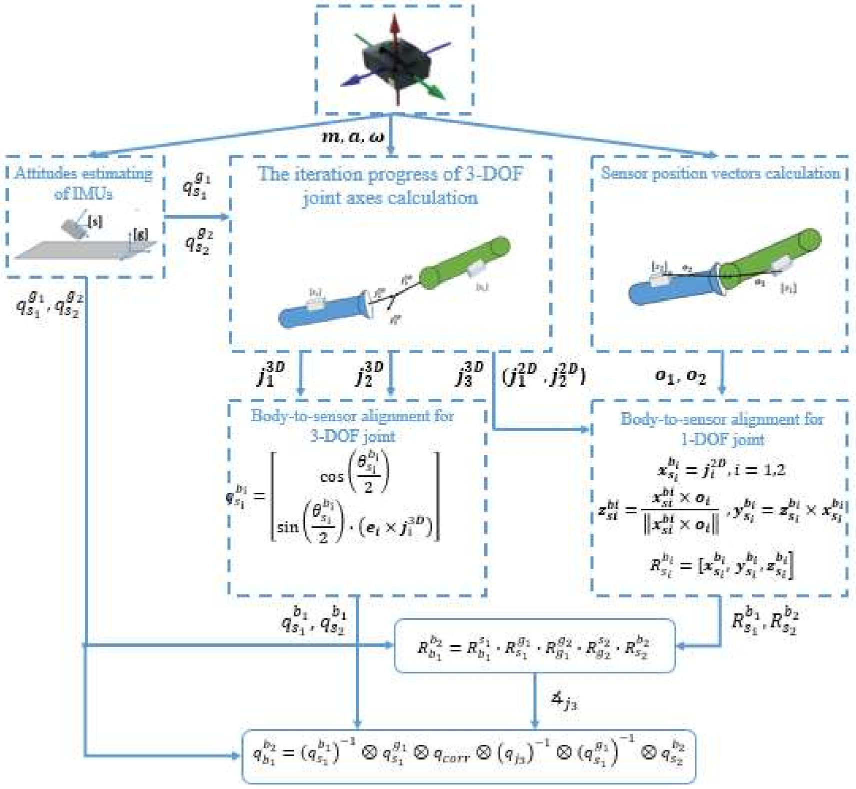


Fig. S2 The flow diagram of the whole 3-D angle estimating algorithm.

TABLE. S1 RMS ERRORS AND CORRELATION COEFFICIENT OWER-LIMB JOINT ANGLES

| | Stair Ascent | | | Squat | | | Level Walking | | |
|---|---|---|---|---|---|---|---|---|---|
| | Flex/Ext | Abd/Add | InR/ExR | Flex/Ext | Abd/Add | InR/ExR | Flex/Ext | Abd/Add | InR/ExR |
| **Hip** | $RMSE_{FE}^{Hip}$(0.99) | $RMSE_{AB}^{Hip}$(0.98) | $RMSE_{IR}^{Hip}$(0.98) | $RMSE_{FE}^{Hip}$(0.99) | $RMSE_{AB}^{Hip}$(0.96) | $RMSE_{IR}^{Hip}$(0.98) | $RMSE_{FE}^{Hip}$(0.99) | $RMSE_{AB}^{Hip}$(0.98) | $RMSE_{IR}^{Hip}$(0.98) |
| | $1.78 \mp 0.78$ | $2.57 \mp 1.27$ | $1.53 \mp 0.59$ | $2.18 \mp 1.45$ | $1.83 \mp 0.73$ | $1.28 \mp 0.21$ | $1.72 \mp 0.89$ | $0.52 \mp 0.26$ | $0.74 \mp 0.44$ |
| | 3.2% | 16.1% | 8.2% | 2.3% | 21.4% | 7.3% | 2.5% | 3.9% | 4.0% |
| **Knee** | $RMSE_{FE}^{knee}$(0.99) | $RMSE_{AB}^{knee}$(0.78) | $RMSE_{IR}^{knee}$(0.94) | $RMSE_{FE}^{knee}$(0.99) | $RMSE_{AB}^{knee}$(0.90) | $RMSE_{IR}^{knee}$(0.96) | $RMSE_{FE}^{knee}$(0.99) | $RMSE_{AB}^{knee}$(0.98) | $RMSE_{IR}^{knee}$(0.96) |
| | $2.87 \mp 0.82$ | $4.94 \mp 0.19$ | $2.47 \mp 1.19$ | $2.98 \mp 1.07$ | $3.15 \mp 0.91$ | $2.67 \mp 0.87$ | $1.72 \mp 0.56$ | $1.82 \mp 0.83$ | $0.88 \mp 0.29$ |
| | 3.2% | 27.8% | 11.3% | 3.2% | 16.3% | 9.6% | 3.7% | 4.9% | 2.7% |
| **Ankle** | $RMSE_{FE}^{ankle}$(0.96) | $RMSE_{AB}^{ankle}$(0.92) | $RMSE_{IR}^{ankle}$(0.86) | $RMSE_{FE}^{ankle}$(0.97) | $RMSE_{AB}^{ankle}$(0.98) | $RMSE_{IR}^{ankle}$(0.93) | $RMSE_{FE}^{ankle}$(0.97) | $RMSE_{AB}^{ankle}$(0.94) | $RMSE_{IR}^{ankle}$(0.97) |
| | $1.24 \mp 0.41$ | $1.44 \mp 0.17$ | $0.66 \mp 0.13$ | $3.08 \mp 1.78$ | $2.21 \mp 0.54$ | $0.39 \mp 0.77$ | $1.34 \mp 0.71$ | $0.44 \mp 0.13$ | $0.72 \mp 0.20$ |
| | 6.0% | 15.1% | 12.8% | 9.1% | 38.3% | 6.6% | 3.5% | 8.1% | 2.5% |

Fle/Ext, Abd/Add and InR/ExR denote Flexion/Extension, Abduction/Adduction and Intro/Extra Rotation respectively. The decimals in brackets denote correlation coefficients of each joint. Numbers after $\mp$ denote the standard deviation of RMSE among subjects.

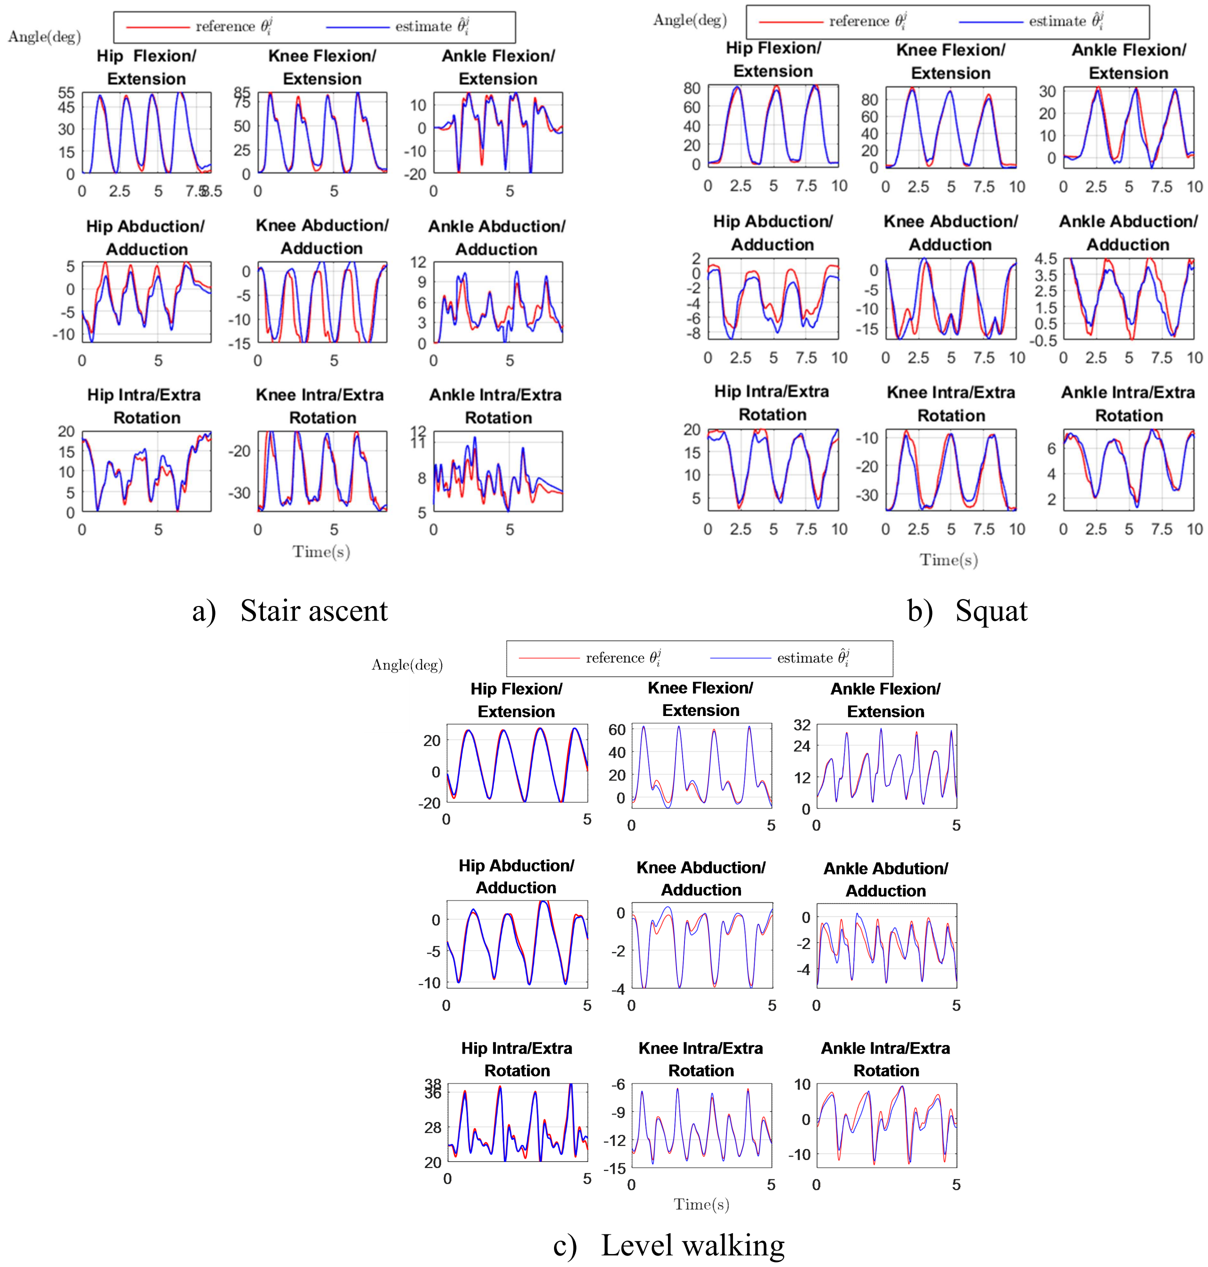


Fig. S3 A comparison between estimated and reference angles on human subjects.

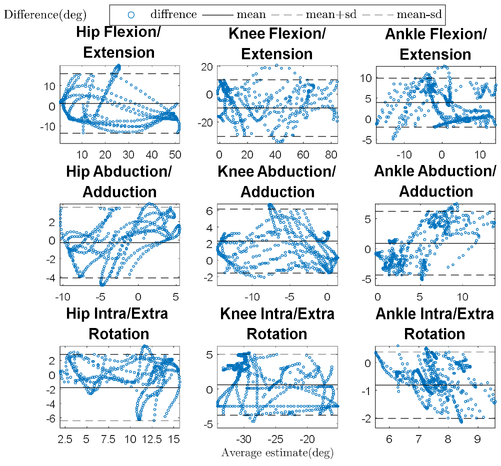


a) Star ascent

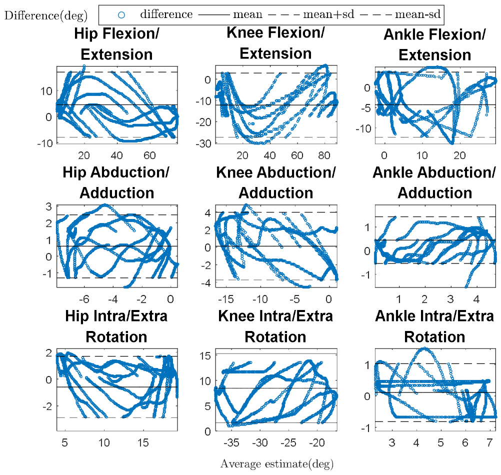


b) Squat

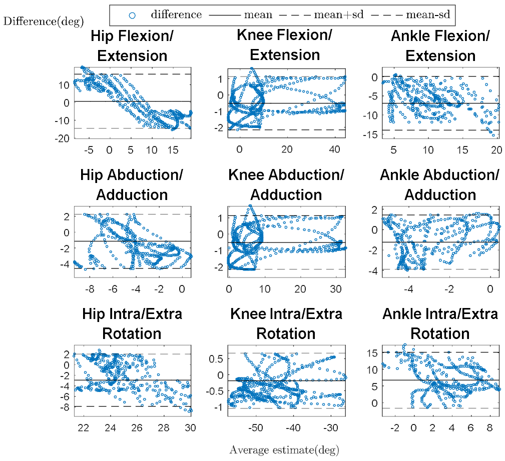


c) Level walking

Fig. S4 The repeatability represented by the difference-average estimates

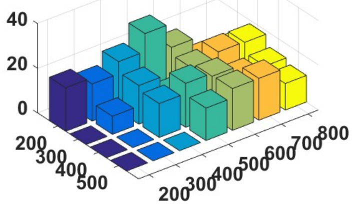

c) Walking

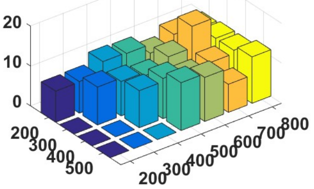

b) Stair ascent

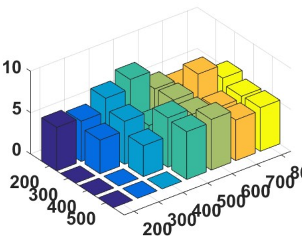

a) Squat

Fig. S5 The comprehensive error metric of the overall effect caused by different sliding windows and intervals.

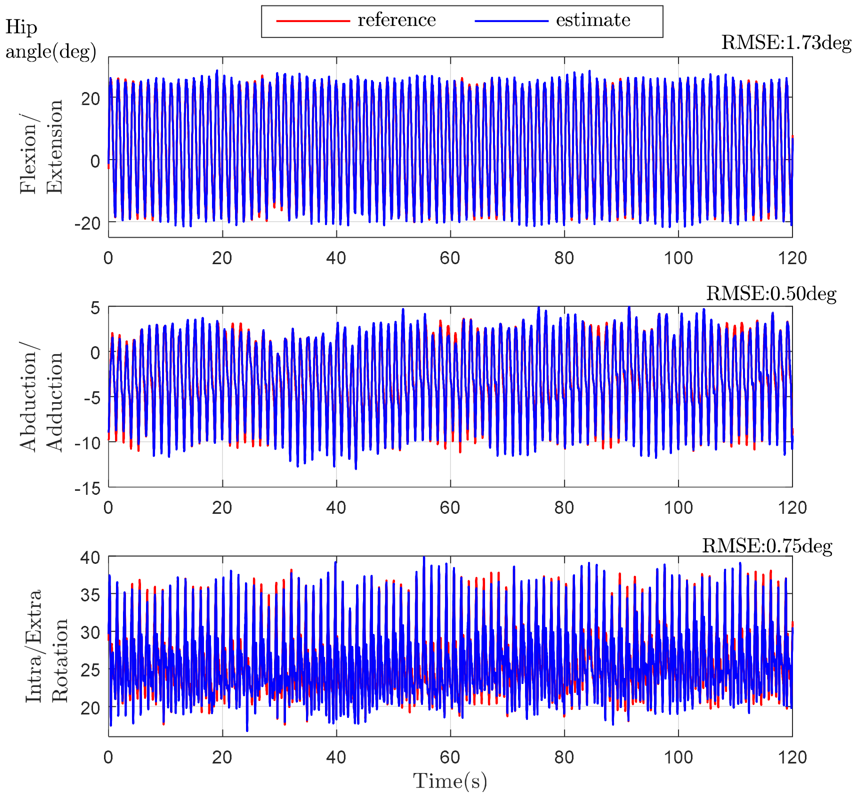
reference
estimate
Hip
angle(deg)
RMSE:1.73deg
Flexion/
Extension
RMSE:0.50deg
Abduction/
Adduction
RMSE:0.75deg
Intra/Extra
Rotation
Time(s)

b) Hip

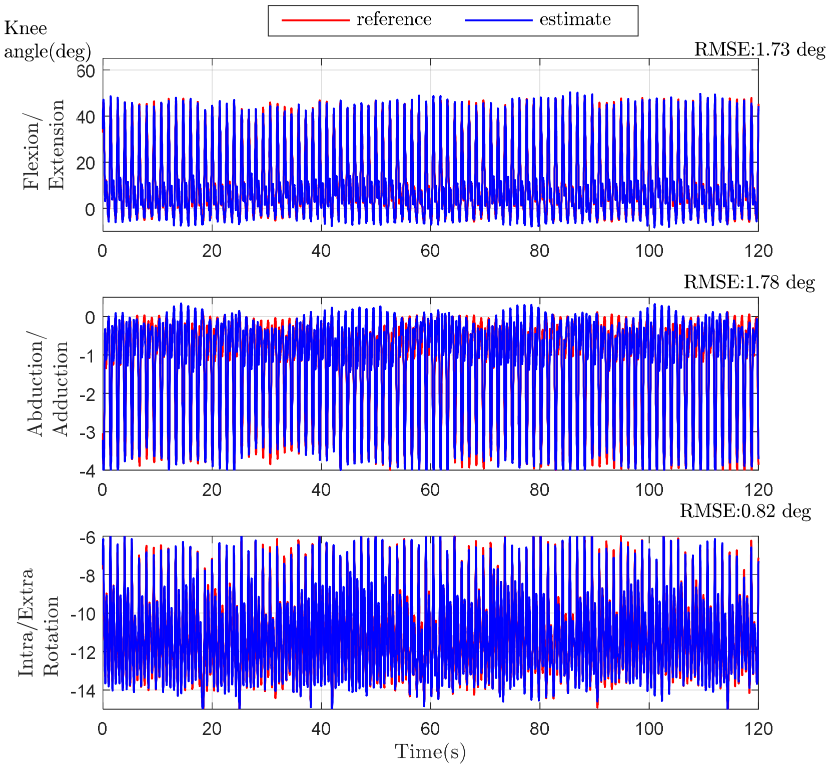
reference
estimate
Knee
angle(deg)
RMSE:1.73 deg
Flexion/
Extension
RMSE:1.78 deg
Abduction/
Adduction
RMSE:0.82 deg
Intra/Extra
Rotation
Time(s)

a) Knee

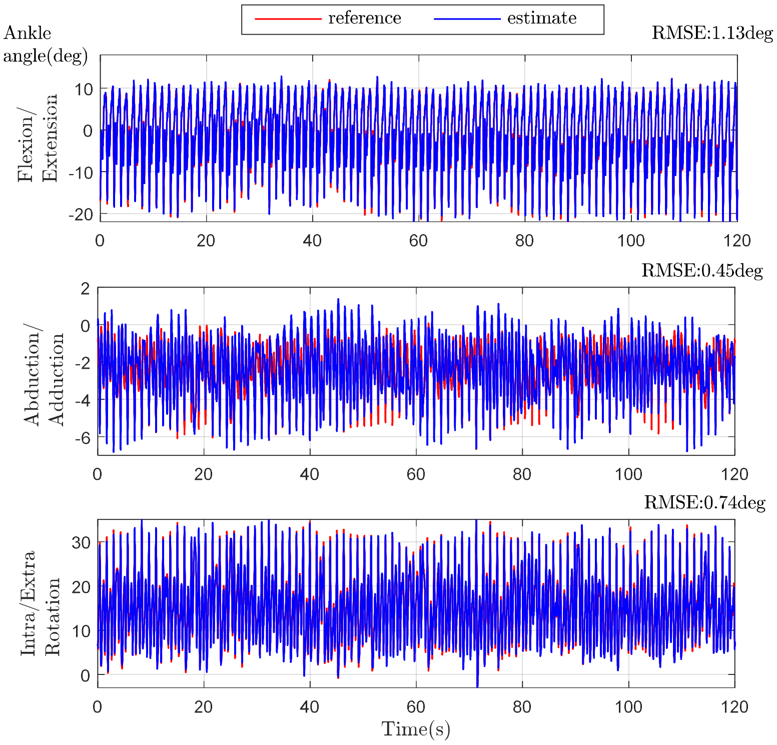


c) Ankle

Fig. S6 The representative figure of 2-min test on level walking.

## 2. Extension to a 3-DOF joint without ~~a~~ main axis

The data processing and analysis mentioned in the manuscript are based on the assumption that a main axis exists during the random movements of the 3-DOF joint. One question of interest is how the algorithm performs without main axis. To answer this question, an experiment was constructed on the gimbal while the magnitudes of angles around all the three axes were ensured to be similar. In this extended experiment, data were processed without considering real-time capability. The length of intervals were set to be as small as possible to compensate the gap caused by processing data in a sliding window.

In this extended experiment, data were processed without considering real-time capability. The length of intervals were set to be as small as possible to compensate the gap caused by processing data in a sliding window, which is shown in Fig. S7.

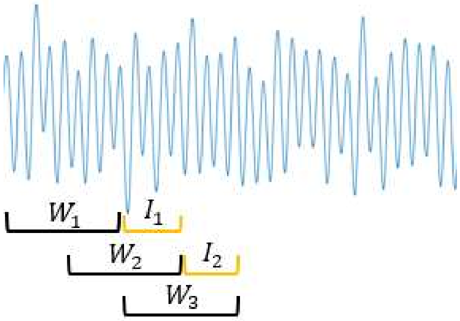


Fig. S7 Data windowing scheme in the extended experiment

The performance of our algorithm on a 3-DOF joint without main axis is depicted in Fig. S8, while the RMS errors of estimates around each axis are also presented. The sliding window is 50 sample points. With 10 sample points of new measurement, the algorithm will be executed to update the joint estimation. To compensate the step and computing time, the length of interval is set to 20 sample points.

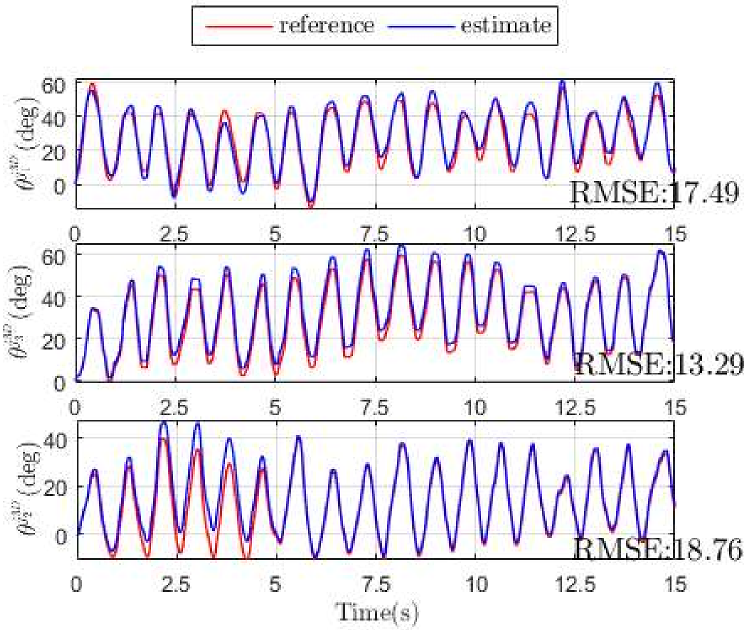


Fig. S8 The performance on a 3-DOF joint without main axis

As shown in Fig. S8, the accuracy reduces severely when there is no main axis existed during the movements. The existence of a main axis ensures that the descent process could lead to an explicit solution. In this experiment, a much smaller sliding window is adopted to make a faster update for joint axis estimation. However, the result shows the accuracy still suffer from errors caused by the delay of joint axis updating. Compared with the experiments on human subjects, a convergence toward an approximate solution is well obtained with a much smaller sliding window. This might result from the smaller acceleration and inexistence of skin artificial movements.
